# Supplementary material for: Experimental Evidence for a Structural-Dynamical Transition in Trajectory Space
Source: arXiv:1609.00327 ancillary file (2017-05-12)
Supplement: Supplementary file 1 [file SupplementalMaterial.pdf]

**Supplementary Material**

# Experimental Evidence for a Structural-Dynamical Transition in Trajectory Space


Rattachai Pinchaipat,[1,2] Matteo Campo,[3,4] Francesco Turci,[1,2]
James E. Hallett,[1,2] Thomas Speck,[4] and C. Patrick Royall[1,5,2,6]

[1]*H.H. Wills Physics Laboratory, Tyndall Avenue, Bristol, BS8 1TL, UK*
[2]*Centre for Nanoscience and Quantum Information, Tyndall Avenue, Bristol, BS8 1FD, UK*
[3]*Graduate School Materials Science in Mainz, Staudinger Weg 9, 55128 Mainz, Germany*
[4]*Institut für Physik, Johannes Gutenberg-Universität Mainz, Staudingerweg 7-9, 55128 Mainz, Germany*
[5]*School of Chemistry, University of Bristol, Cantock's Close, Bristol, BS8 1TS, UK*
[6]*Department of Chemical Engineering, Kyoto University, Kyoto 615-8510, Japan*


## I. EXPERIMENT DETAILS

Poly-methyl methacrylate (PMMA) colloids, sterically stabilised with poly(12-hydroxy stearic acid) were used as a model system. Particle size and polydispersity were determined using scanning electron microscopy (SEM) (JSM-5600LV, JEOL). The particle diameter $\sigma$ was 1.981$\pm$0.155 $\mu$m and the polydispersity was 8%, sufficient to suppress crystallisation. The particles were fluorescently labelled throughout with rhodamine-B and suspended in a density and refractive index matched solvent mixture. A mixture of cis-decalin and bromocyclohexane (CHB) (27/%w/w) was used, and any surface charge was also screened by adding 4 mM of tetra butyl ammonium bromide (TBAB).

The density and refractive index matched samples were placed in square capillaries with internal side of 500 $\mu$m (Vitrotubes) and both ends were sealed with epoxy. Samples were then left to equilibrate for 12 hours. Confocal microscopy was performed using a Leica SP5 microscope with room temperature fixed at $20 \pm 0.2°$ C. We imaged at least 40 $\mu m$ from the wall. The effective volume fraction $\phi$ was obtained by reference to the dynamical behavior compared with simulation data as described below. We obtain the particle coordinates using the "Colloids" tracking code [1]. Our methodology is shown in Supplementary Fig. S1. Typically, around 10,000 particles are analysed in each 3d image and tracked in time.

## II. STRUCTURAL ANALYSIS AND THE EFFECT OF TRACKING ERRORS

Our structural analysis for both experiment and simulations rests upon identifying the locally favoured structures in the coordinate data. This we do using the topological cluster classification (TCC), which performs a Voronoi decomposition to define a bond network between the particle coordinates. Local bond networks are identified and

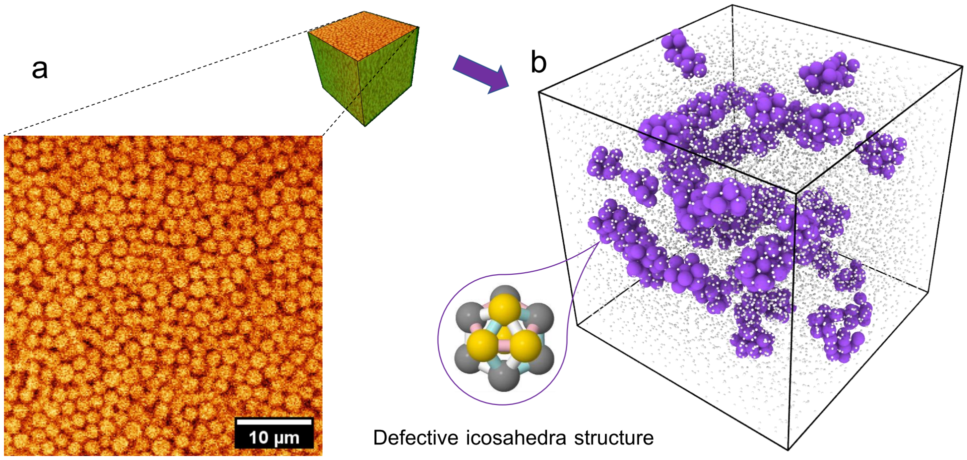


FIG. S1: Extracting locally favored structures from particle-resolved studies at $\phi = 0.58$. (a) 2d cross section confocal image taken from a 3d data set as indicated. (b) Particle coordinates tracked in a 3d confocal image. Those rendered in purple are identified as defective icosahedra LFS by the topological cluster classification [2]. Small grey particles are not identified as LFS.

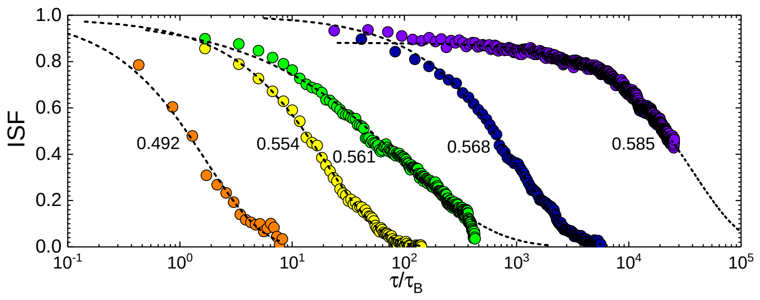


FIG. S2: Experimental intermediate scattering functions $F(k, t)$. for a range of effective volume fractions as indicated. The data are fitted with a stretched exponential as indicated by the dashed lines.

their topology compared with bond networks for certain geometric motifs, in this case the ten-membered defective icosahedron. This has been identified as the locally favoured structure in hard spheres [3]. Further details of the method may be found in [2]. Here we cut off neighbouring particles at a separation of 1.4 $\sigma$ and an $f_c$ parameter of 0.87 [2] was chosen to limit the selectivity of the TCC identification algorithm in the experimental data to the tracking errors. The effect of reducing the fraction of LFS due to tracking errors is shown in Fig. 1(b) in the main text.

To determine the effect of tracking errors on the LFS population, we assume that they are Gaussian distributed. We therefore add such errors to a set of co-ordinates from our bulk simulation data. The Gaussian had a standard deviation of $0.05\sigma$. The results are shown in Fig. 1(b).

## III. DYNAMICAL ANALYSIS

The intermediate scattering function (ISF) $F(k, t)$ was determined from a time series of particle coordinates for both experimental and simulation data:

$$F(t) = \frac{1}{N} \left\langle \sum_{j=1}^{N} \exp\left(2\pi i/\sigma \cdot (\boldsymbol{r}_j(t) - \boldsymbol{r}_j(0)\right) \right\rangle \tag{1}$$

where $\boldsymbol{r}$ is the particle position and $\sigma$ is the average particle diameter. The structural relaxation time $\tau_\alpha$ was obtained by fitting the ISF with a stretched-exponential decay using the Kohlrausch-Williams-Watts (KWW) expression $F(\mathbf{k}, t) = c \exp\left[-(t/\tau_\alpha)^b\right]$. In this way, the relaxation time was determined for each state point as shown in Fig. S2, and then compared with the results from simulation by rescaling $\tau_\alpha$ with the Brownian time ($\tau_B$), which is defined as the time that a particle can diffuse a distance of one diameter in the dilute limit. We measured the diffusion coefficient $D$ from the mean square displacement

$$\langle \Delta r(t)^2 \rangle = \langle (\boldsymbol{r}(t) - (\boldsymbol{r}(0))^2 \rangle = 6Dt \tag{2}$$

at low volume fraction ($\phi \sim 0.01$). This gives us the diffusion coefficient from the definition of the MSD and $\tau_B = \bar{\sigma}^2/D$. Note that in Fig. S2, the ISFs do not fully decay. This is due to the difficulty in obtaining coordinate trajectories of sufficient length in the experiments. While this gives some uncertainty as to the long-time behaviour of the ISF we emphasise that the experiments are equilibrated for at least 30 $\tau_\alpha$, so we expect the system to be well equilibrated for our purposes, and that the decay we see is consistent with that obtained from simulation data [4].

Accurately determining the effective volume fraction $\phi$ in colloidal systems is a challenging matter [5, 6]. This is particularly important in dynamical arrest where the dynamical properties of interest change so drastically over a small change in volume fraction. However this very sensitivity of, for example the structural relaxation time, means that it can be used as a rather accurate means by which to calibrate the effective volume fraction when benchmarked against simulations. We recall that for supercooled systems, the type of dynamics used in the simulation is not important when determining the relaxation time [7], and hydrodynamics enables the long-time self-diffusion to be rescaled [8]. We therefore rescale our experimental volume fractions to our simulation data in Fig. 1(a) in the main text.

## IV. FITTING THE LFS POPULATION

In the case of the structural-dynamical phase transition in Fig. 2(a-c), we wish to estimate the volume fraction that the LFS-rich phase corresponds to. To do so, we seek an expression for the LFS population as a function of volume fraction, $n_{\mathrm{LFS}}(\phi)$. Now the LFS population increases quite steeply as a function of $\phi$, so we find it convenient to use the compressibility factor $Z$ instead. We take this to be related to the volume fraction by the Carnahan-Starling relation

$$Z = \frac{1+\phi+\phi^2-\phi^3}{(1-\phi)^3}. \tag{3}$$

We fit the experimental population of LFS to $Z$ with the following expression

$$n_{\mathrm{LFS}} = \frac{1}{(1+B/Z)^{\delta}} \tag{4}$$

where $B$ and $\delta$ are constants determined by fitting the data. For the experimental data, $B = 27.41$ and $\delta = 6.463$, and for the simulations $B = 21.19$ and $\delta = 5.954$. In Fig. 1(b) in the main text, the dashed and solid grey lines are Eq. 4 with experimental and simulation parameters respectively. We then use Eqs. 3 and 4 to estimate the volume fractions the LFS-rich phase corresponds to in Fig. 1(b). We emphasize that this form is merely chosen to be a convenient means to fit the data and do not wish to imply any physical motivation.

## V. TRAJECTORY ANALYSIS

To investigate the dynamical phase transition, we seek to identify LFS populations along trajectories. These trajectories we then bin into a histogram according to the population of particles in LFS along the trajectory. In the case of the biased simulations, the raw data is the trajectories, but in the case of the larger bulk unbiased simulations, and the experiments, we need to *subsample* the trajectories from the larger system.

To subsample the bulk simulations, we select a centre particle and define the trajectory as the nearest $N-1$ particles to it, or a trajectory of $N$ particles. In the case of the experiments, due to tracking errors there may be occasional particles missing in some frames which act to truncate trajectories so we therefore modified our trajectory analysis by defining spatial boundaries around particles at t=0 such that $N = 100$ particles were enclosed. This spatial region (rather than the number of particles as for the simulation data) then defined the trajectory. We checked this change had no effect on the results by determining the distributions for simulation data with both definitions for the trajectory and found no meaningful difference.

We count the number of defective icosahedra in the cell (yellow shaded sphere, Fig. 3 (main text), along 10 time steps (of duration 0.97 $\tau_\alpha$). The subsampled coordinates within this sphere consist of $\approx 100$ particles and the centres of the boundaries coincide with the particle positions at t=0. We then produce a histogram of the fractions of particles in defective icosahedra LFS from these trajectories.

## VI. TRAJECTORY ANALYSIS FOR THE DYNAMICAL $s$-ENSEMBLE

*Experiment.* — We performed the analysis for the dynamical, $s-$ensemble as follows. Briefly, the $s-$ensemble considers distributions of trajectories, and identifies a "fat-tail" of trajectories with very slow dynamics as evidence of a dynamical transition [9, 10]. Here we seek such a distribution, but for the case of the coordinates tracked in experiments, this is hampered due to particle tracking errors [5] which we estimate as 5% of the diameter [see Fig. 1(b) in the main text], which places a "noise floor" on the displacements which can be measured.

We therefore implemented a different method to analyse the data. In particular, the analysis is based on confocal differential dynamic microscopy (ConDDM) [11, 12]. This technique rests on the observation that, for small displacements, the sum of square of differences of intensity between images at time $t$ and $t+\delta t$, $\Sigma_i(I(t+\delta t)-I(t))^2$ is proportional to the displacement of particles. Here $i$ runs over the pixels in the image. Supplementary Fig. S3 shows the relationship between displacements and intensity differences. In Supplementary Fig. S3(a), we show a binarised

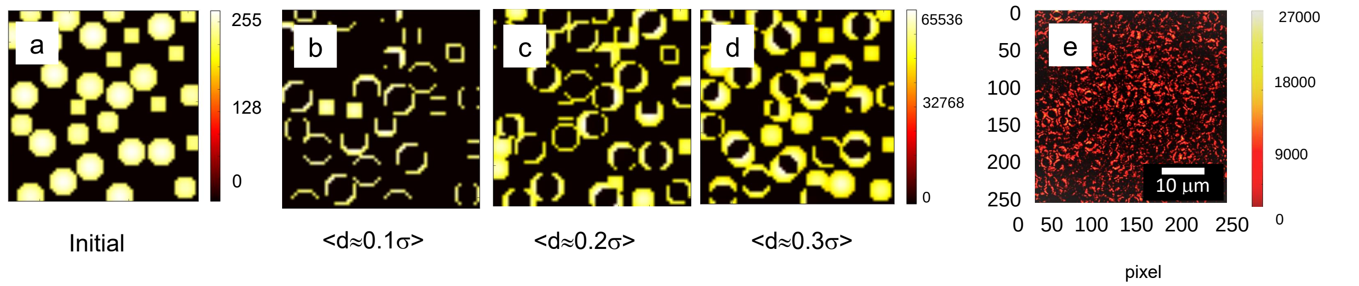


FIG. S3: Dynamical analysis with confocal differential dynamic microscopy. (a) Cross section of 3D simulation image (shown in $xy$) at $\phi = 0.44$. (b),(c) and (d) The square of the difference in intensity when the simulated particles have moved an average displacement of $0.1\sigma$,$0.2\sigma$ and $0.3\sigma$. (e) The crossection of the squared value of the difference in intensity between 2 images seperated by a time difference 0.2 $\tau_\alpha$. Data shown is 2d slice from 3d image at $\phi = 0.58$.

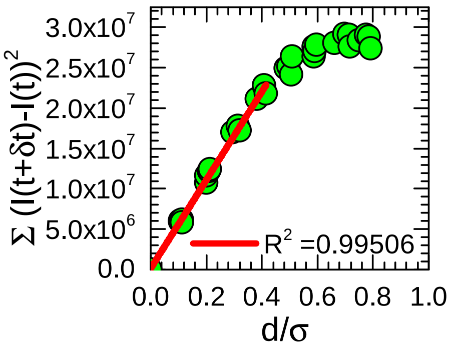


FIG. S4: Linearity of square of difference in intensity vs average displacement. Here $d$ is determined from particle coordinate data.

image, to schematically illustrate the process. This binarised image uses simulated data at $\phi = 0.3$. Panels (b-d) then illustrate the sum of squares as the mean displacement of the particles is $0.1\sigma$,$0.2\sigma$ and $0.3\sigma$ respectively. The method is shown in action in panel (e).

From Fig. S4, we see that when the average displacement of particles is less than around 0.4 $\sigma$, the sum of the square of differences of intensity exhibits the same scaling as the mean square displacement. We thus obtain a means to determine smaller displacements than can be reliably accessed from coordinate data.

To relate the DDM data to the dynamical heterogeneity which underlies the dynamical transition, we use the position of particles in the first frame as a reference for drawing a sphere boundary of radius $2.87\sigma$ which is equivalent to the sphere which contains $\approx 100$ particles as used for the trajectory analysis for the $\mu-$ensemble described in the main text. This is shown in Fig. S5. For each initial position (*i.e.* trajectory) we sum the square of the difference between intensity at $t + \delta t$ and $t$ inside the sphere boundary along the time difference $\delta t \approx 0.2\tau_\alpha$. We integrate $\Sigma_i$

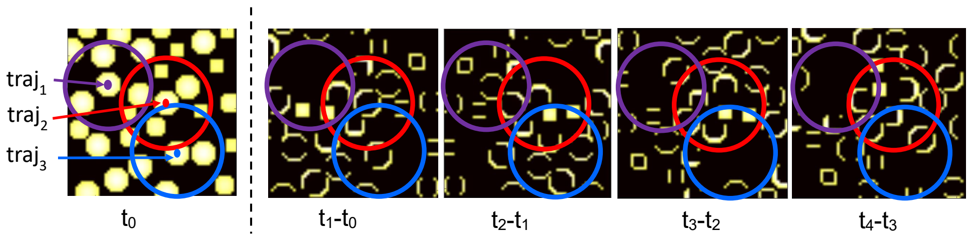


FIG. S5: Illustration of trajectory analysis of the DDM data, as described in the text. Circles represent spheres of radius $2.87\sigma$.

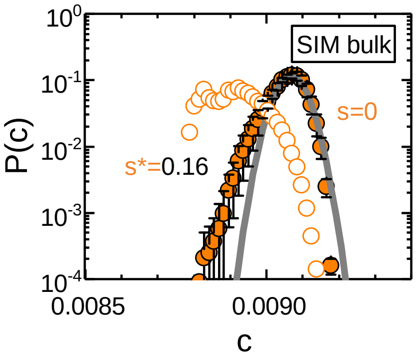


FIG. S6: Distribution of trajectory mobilities at $s = 0$ (filled circles) and $s^* = 0.16$ (unfilled circles) over a trajectory length of ≈6.5 $\tau_\alpha$. This figure is analogous to Fig. 4(e) in the main text. The continuous line is a Gaussian fit to the data.

along trajectories of comprised of $K$ images of length $1\tau_\alpha$.

$$C_{\rm dmm} = \sum_k \left(\Sigma_i (I(t+\delta t) - I(t))^2\right) \tag{5}$$

Then the total sum was divided by the maximum intensity $I_{\rm max}$ and number of pixels in the image $n_{\rm pix}$. We define this normalised mobility $c_{\rm ddm} = C_{\rm dmm}/(KI_{\rm max}n_{\rm pix})$. Finally, we plot the histogram of $c_{\rm ddm}$ to represent evidence of a dynamical transition in trajectory space as Fig. 2(e) in the main text.

To reveal the dynamical transition, we then reweight the trajectories in an analogous way to the $\mu$ field as described in Eq. (1) in the main text. We consider the order parameter $c_{\rm ddm}$ and the dynamical field $s$:

$$P_s(c_{\rm ddm}) \propto P(c_{\rm ddm})\ \exp[-sc_{\rm ddm}N(K+1)] \tag{6}$$

*Simulation.* — In simulation we consider the mean squared displacement from coordinate data, similar to previous work [9]. To confirm that the dynamical transition is found in sub-sampled unbiased data, analogous to Fig. 2(b) in the main text, we show the distribution of trajectory mobilities in Fig. S6. Here we define the mobility as the time-integrated mean square displacement per particle in a trajectory of length $5\tau_\alpha$.

The analysis was performed following [13]. We follow particle trajectories and then count the number of mobile particles among the closest 99 particles. We define $h^m_k(t) = \Theta(|\hat{\mathbf{r}}_k(t) - \hat{\mathbf{r}}_k(t-\delta t)| - a)$, where $\Theta$ is the Heaviside step function. Thus $h^m_k(t) = 1$ when a particle moves further than $a = 0.1\sigma$ in duration $\delta t = 0.33\tau_\alpha$. Otherwise it is 0. Then we integrate $C$ along time $t \approx 6.5\tau_\alpha$. $C = \sum_{ik} h^m_k(t_i)$ where $k = 1, 2, ..100, i = 1, 2, 3, ..K$. The mobility $c$ is defined as $c = C/NK$ where N=10976, K=20. We then plot the histogram of mobility as shown in Fig. S6.

## VII. RELATING THE STRUCTURAL-DYNAMICAL TRANSITION TO THE SPECIFIC LOCAL STRUCTURE

It is important to confirm that the structural-dynamical phase transition we find is related to the locally favoured structure, the defective icosahedron. In Fig. S7, we show that upon carrying out the same analysis as that in Fig. 2(a) in the main text, a Gaussian distribution of time-integrated structure populations is found along the trajectories. This indicates that the structural-dynamical transition considered in the main text is indeed related to the defective icosahedron LFS.

## VIII. BIASED SIMULATION DETAILS

We perform a random walk through the space of trajectories according to a distribution $P(x)$ of trajectories $x$. Each trajectory is generated using event-driven molecular dynamics for the five-component system described in the main text but at a slightly higher polydispersity of 10% obtained through scaling particle diameters. To carry out the random walk in trajectory space, we need to satisfy the detailed balance

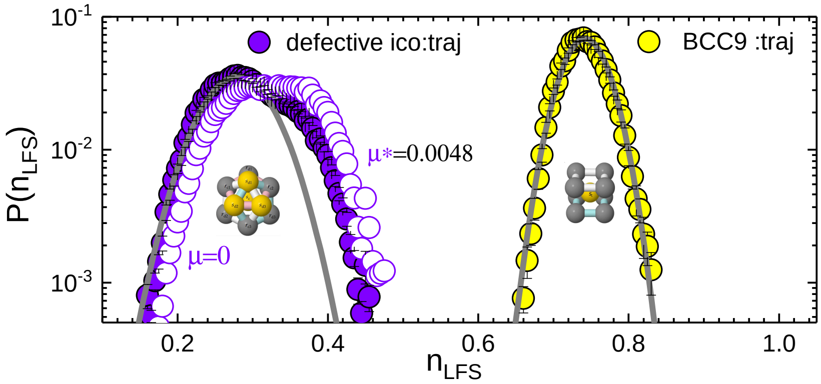


FIG. S7: Analysis of trajectories with a nine-membered structure with four-fold symmetry distinct to the LFS. No evidence of a structural-dynamical phase transition is found.

$$P(o)P_{\text{gen}}(o \to n)P_{\text{acc}}(o \to n) = P(n)P_{\text{gen}}(n \to o)P_{\text{acc}}(n \to o) \tag{7}$$

where $o$ and $n$ are the old and the new trajectories, $P_{\text{gen}}(o \to n)$ is the probability of generating $n$ from $o$, and $P_{\text{acc}}(o \to n)$ is the probability of accepting it.

The probability of acceptance is determined by the Metropolis Criterion

$$P_{\text{acc}}(o \to n) = \min\left[1, \frac{P(n)P_{\text{gen}}(n \to o)}{P(o)P_{\text{gen}}(o \to n)}\right] \tag{8}$$

which ensures the detailed balance is preserved.

The generation probability is determined by the kind of Monte Carlo move which is used to obtain a new trajectory from an old one. We employ two moves from transition path sampling TPS [14], shifting and shooting with a ratio of 0.25 between the two. It can be easily shown that using these moves and choosing $P(x) = P_0(x)e^{-\omega(x)}$ lead to the simple acceptance rule

$$P_{\text{acc}}(o \to n) = \min\left[1, \frac{e^{-\omega(n)}}{e^{-\omega(o)}}\right] \tag{9}$$

The shape of $\omega$ is chosen to be parabolic

$$\omega(x) = \frac{1}{2}k(n_{\text{LFS}}[x] - n_0)^2 \tag{10}$$

where $n_{\text{LFS}}[x]$ is the average fraction of particles in defective icosahedra along the trajectory $x$, as measured with the TCC [2]. The purpose of $\omega$ is to bias the sampling towards trajectories with $n_{\text{LFS}} \simeq n_0$. We use replica exchange between 16 replicas with different values of $n_0$, spanning the range $0.25 < n_0 < 0.75$.

The typical Monte Carlo step will thus be: generation of a new trajectory for each replica using shifting/shooting moves; acceptance or rejection of each newly created trajectory; swap of trajectories between all the replicas (not only between neighbours). The Monte Carlo simulation is let to equilibrate for a number $N_{\text{eq}}$ of cycles before the data is collected. The equilibration can be checked by looking at the order parameter $n_{\text{LFS}}$ for each individual replica. The Monte Carlo simulation reaches equilibrium after around $10^3$ steps and we start collecting data after $N_{\text{eq}} = 5 \times 10^3$ MC steps. To finally obtain the distribution $n_{\text{LFS}}$, we combine the data obtained from all the replicas by using the Multistate Bennet's Acceptance Ratio (MBAR) method extended to ensembles of trajectories [15].

[1] M. Leocmach and H. Tanaka, Soft Matter **9**, 1447 (2013).

[2] A. Malins, S. R. Williams, J. Eggers, and C. P. Royall, J. Chem. Phys. **139**, 234506 (2013).
[3] C. P. Royall, A. Malins, A. J. Dunleavy, and R. Pinney, J. Non-Cryst. Solids **407**, 34 (2015).
[4] C. P. Royall and W. Kob, accepted J. Stat. Mech.: Theory and Experiment, online at AXiV 1611.03314 (2016).
[5] W. C. K. Poon, E. R. Weeks, and C. P. Royall, Soft Matter **8**, 21 (2012).
[6] C. P. Royall, W. C. K. Poon, and E. R. Weeks, Soft Matter **9**, 17 (2013).
[7] L. Berthier and R. Jack, Phys. Rev. E **76**, 041509 (2007).
[8] A. L. Thorneywork, R. E. Rozas, R. P. A. Dullens, and J. Horbach, Phys. Rev. Lett. (2015).
[9] L. O. Hedges, R. L. Jack, J. P. Garrahan, and D. Chandler, Science **323**, 1309 (2009).
[10] D. Chandler and J. P. Garrahan, Annual review of physical chemistry **61**, 191 (2010).
[11] P. J. Lu, F. Giavazzi, T. E. Angelini, E. Zaccarelli, F. Jargstorff, A. B. Schofield, J. N. Wilking, M. B. Romanowsky, D. A. Weitz, and R. Cerbino, Phy. Rev. Lett. **108**, 1 (2012).
[12] R. Cerbino and V. Trappe, Phy. Rev. Lett. **100** (2008).
[13] T. Speck, A. Malins, and R. C. P., Phys. Rev. Lett. **109**, 195703 (2012).
[14] P. G. Bolhuis, D. Chandler, C. Dellago, and P. L. Geissler, Annual review of physical chemistry **53** (2002).
[15] D. D. L. Minh and J. D. Chodera, J. Chem. Phys. **131**, 134110 (2009).
